# Supplementary material for: Unconventional superconductivity induced by suppressing an iron-selenium based Mott insulator CsFe4-xSe4
Source: arXiv:2008.12191 source file (2020-08-27)
Supplement: Supplementary file 1 [file CsFe4Se4_supplementary_2ndv3.pdf]

# Supplementary Information

# Superconductivity induced by suppressing an iron-selenium based Mott insulator $CsFe_{4-x}Se_4$

Jin Si, Guan-Yu Chen, Qing Li, Xiyu Zhu, Huan Yang and Hai-Hu Wen*

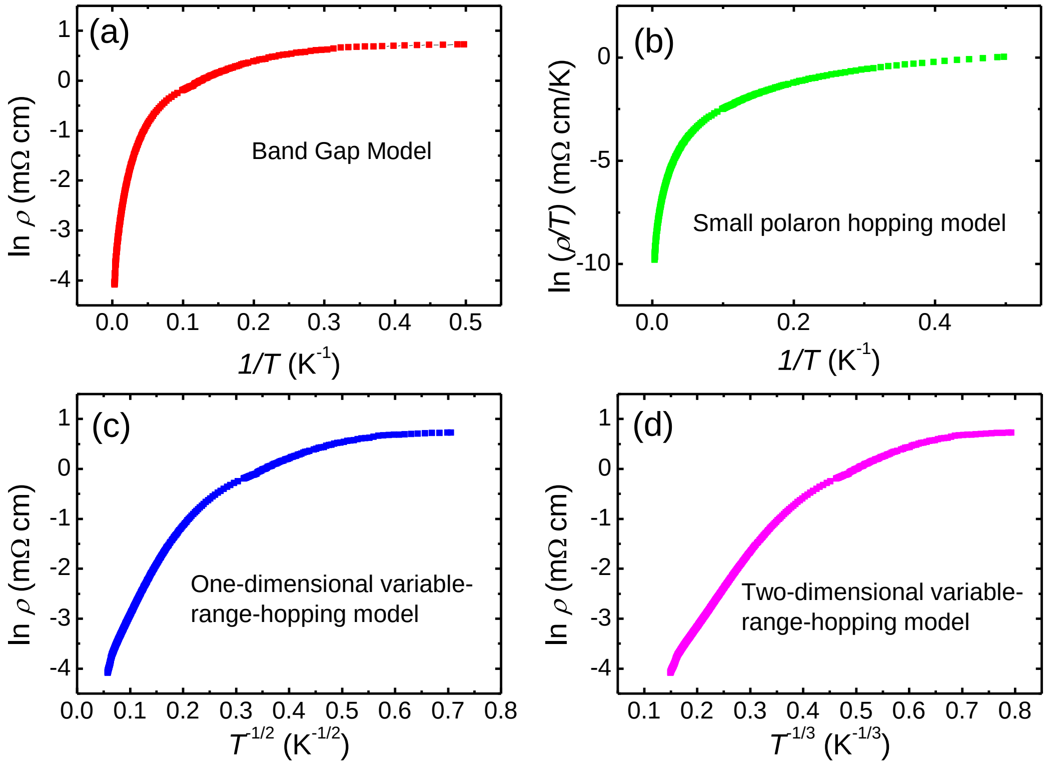


Figure S1: Several models adopted to fit the resistivity data. (a), Band gap model. (b), Small polaron hopping model. (c), One-dimensional variable-range-hopping model. (d), Two-dimensional variable-range-hopping model. All above models fail to describe the resistivity of $CsFe_{4-x}Se_4$.

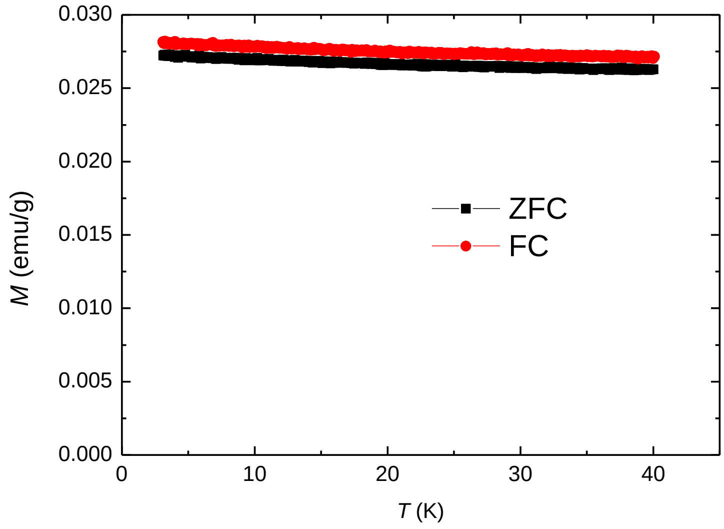


Figure S2: The low-temperature M (T) curves at H = 10 Oe with ZFC and FC modes. From the data, we can confirm the absence of superconducting phases like FeSe and $CsFe_2Se_2$ in as-prepared $CsFe_{4-x}Se_4$ at ambient pressure. The slight difference of M (T) curves between ZFC and FC modes is attributed to the tiny amount of Fe impurity.

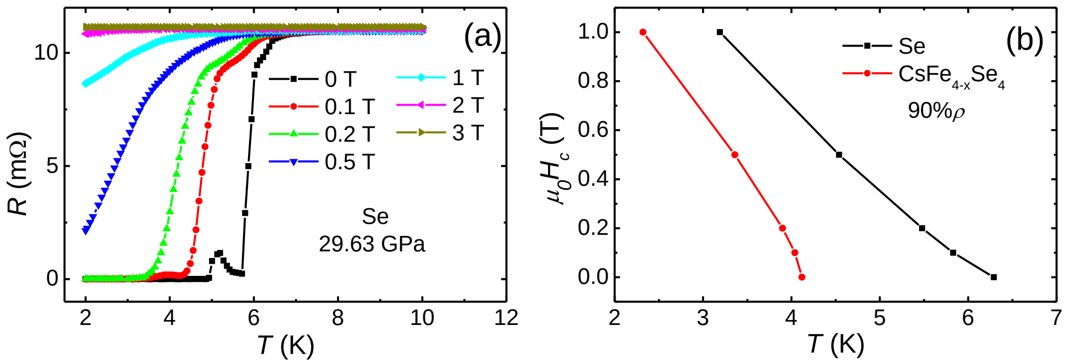


Figure S3: Comparison between Se and $CsFe_{4-x}Se_4$ at about 30 GPa. (a), The resistivity of Se at 29.53 GPa measured under different magnetic fields. (b), Comparison of upper critical field between Se and $CsFe_{4-x}Se_4$ at about 30 GPa. It is obvious that the superconductivity induced in $CsFe_{4-x}Se_4$ does not come from the elemental Se.

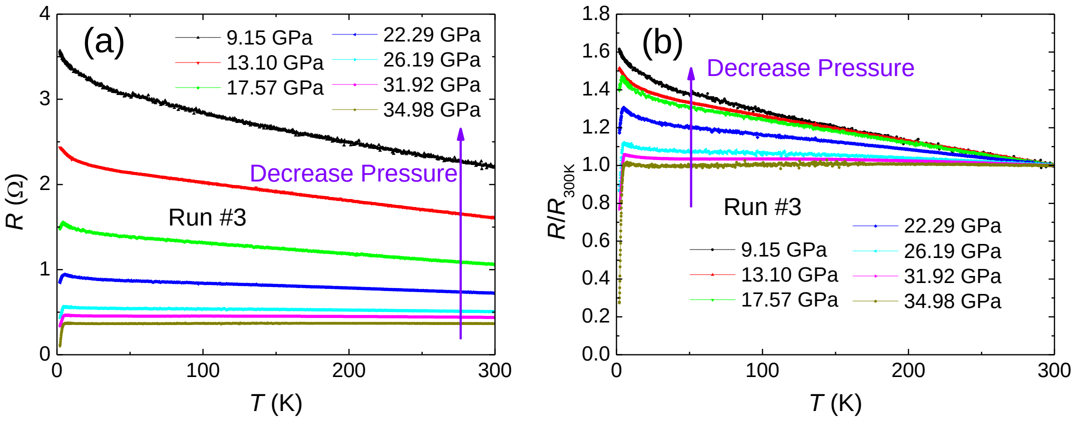


Figure S4: (a), Temperature dependent resistance and normalized resistance at high pressures with decreasing pressure for Run #3. (b), The same data as that in (a) plotted as normalized by resistivity at 300 K.
